# Supplementary material for: Stiffness and atomic-scale friction in superlubricant MoS$_2$ bilayers
Source: arXiv:2107.00486 source file (2021-07-01)
Supplement: Supplementary file 1 [file Supplemental_Material.pdf]

# Supplemental materials to

*Stiffness and atomic-scale friction in superlubricant $MoS_2$ bilayers*

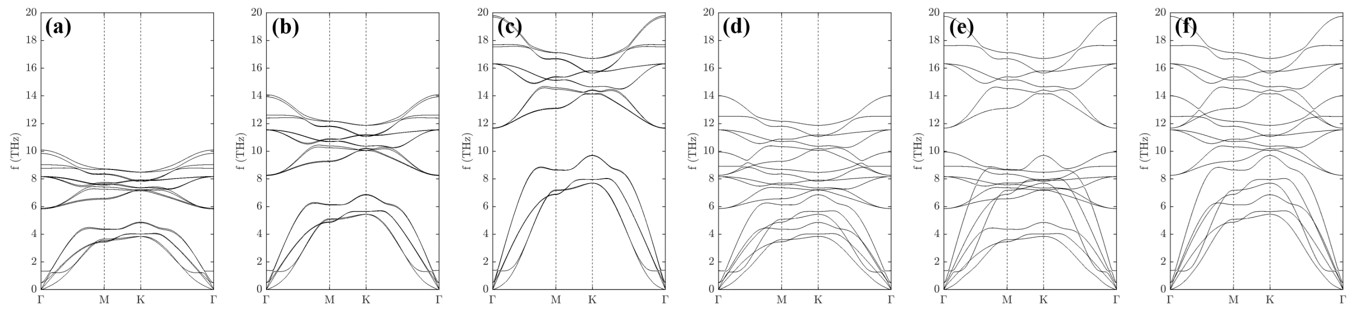


FIG. 1. Phonon spectra of combinations of soft (S), normal (N) and hard (H) $MoS_2$ layers. (a) S-S, (b) N-N, (c) H-H, (d) S-N, (e) S-H and (f) N-H.

The phonon spectra of bilayers are calculated with LAMMPS [1] using the finite different method. A 6×6×1 super-cell is used for the $MoS_2$ bilayer. Each atom in the primitive cell is displaced along the $x$-, $y$- and $z$-axis by 0.01 Å, and the energies are calculated by using our constructed spectral neighbor analysis potential (SNAP) and the inter-layer Lennard-Jones potential, as described in the main text. Fig. 1(a)-(c) present the intra-layer stiffness of soft (S), normal (N) and hard (H) $MoS_2$ bilayers. Fig. 1(d)-(f) show the different level of overlap between the phonon band-structures of hetero-bilayeres. The two lowest modes at Γ are the shear mode (SM) and layer-breathing mode (LBM). One should notice they have the same frequencies for all the six combinations. This provides evidence that the inter-layer sliding energy surface (ISES) are the same.

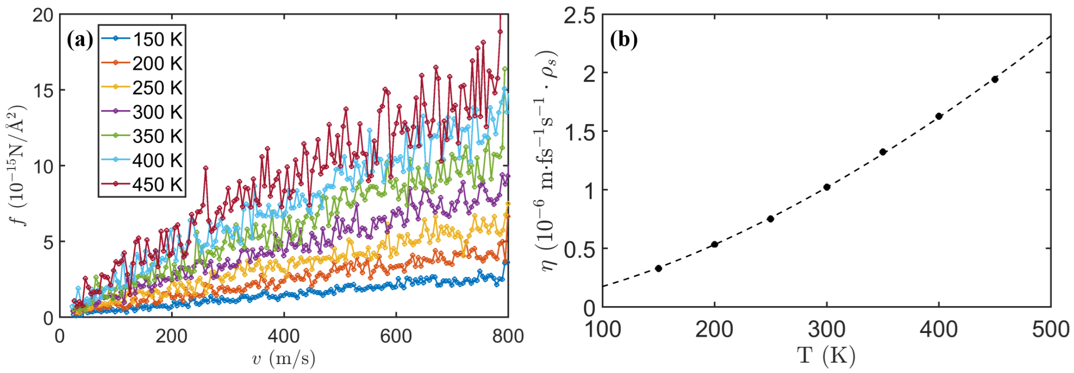


FIG. 2. Temperature dependence of the friction force. (a) $f(v)$ curves for the N-N bilayer at different temperatures. (b) Fit of the viscous coefficient $\eta$ to the power-law model. The solid dots are the values of $\eta$ and the dashed line is the fit, $\eta(T)$.

In order to study how the friction depends on temperature, we simulate the free sliding of the N-N bilayer, where the substrate is thermalized at different temperatures. The substrate temperatures are set to range from 150 K to 450 K in 50 K steps. The friction force is fitted to $f = -\eta(v/v_{\mathrm{ref}})^k$ [see Eq. (1) in the main text]. Here $k$ is set the value at 300 K, namely 0.83, so that $\eta$ is the only parameter left to be determined. This approach eliminates numerical instabilities in the fit and leads to a better comparison between different temperatures. The $\eta(T)$ curve is then fitted again to a power-law $\eta = C \cdot T^n$, and we obtain $n$=1.6.

[1] S. Plimpton, *Fast Parallel Algorithms for Short-Range Molecular Dynamics*, J. Comp. Phys. **117**, 1 (1995).
hbp
